# Supplementary material for: Generative Timelines for Instructed Visual Assembly
Source: arXiv:2411.12293 source file (2024-11-19)
Supplement: Supplementary file 1 [file minigpt4-failure.tex]

\begin{figure*}[h]
    \centering
    \includegraphics[width=0.98\linewidth]{supplementary/images/minigpt4-failure.pdf}

    \caption{\textbf{Timeline Assembler vs. MiniGPT-4 outputs.} The timeline assembler understand the assembly instruction and generates the appropiate timeline. Meanwhile, MiniGPT-4 generates captions of the visual content without understanding the instructed task.}
    \label{fig:minigpt4-failure}
\end{figure*}
