# Supplementary material for: Generative Timelines for Instructed Visual Assembly
Source: arXiv:2411.12293 source file (2024-11-19)
Supplement: Supplementary file 2 [file gpt-task-classifier.tex]

\begin{table}[ht]
\centering
\begin{tabular}{l|c}
\hline
\textbf{Task}           & \textbf{Accuracy} \\ \hline
Positional Insertion  & 78.8\%      \\
Positional Removal    & 100.0\%     \\
Positional Replacement & 78.8\%     \\
Positional Swap       & 75.0\%      \\
Semantic Insertion    & 56.2\%      \\
Semantic Replacement  & 63.8\%      \\
Semantic Removal      & 96.2\%      \\
Semantic Swap         & 25.0\%      \\
\hline
\end{tabular}
\caption{\textbf{GPT-3.5 Task-Classifier Results.}}
\label{tab:gpt-3.5-classifier}
\end{table}
