# Supplementary material for: Generative Timelines for Instructed Visual Assembly
Source: arXiv:2411.12293 source file (2024-11-19)
Supplement: Supplementary file 3 [file implementation_details.tex]

\begin{table}[ht]
\centering
\begin{tabular}{@{}lc@{}}
\toprule
Configuration         & Value \\ \midrule
LoRA - r              & 16 \\
LoRA - $\alpha$         & 32 \\
LoRA - dropout        & 0.1 \\
\midrule
Optimizer             & AdamW \\
Optimizer momentum    & \(\beta_1, \beta_2 = 0.9, 0.999\) \\
Weight decay          & 0.05 \\
Base learning rate    & \(6 \times 10^{-5}\) \\
Warmup learning rate &  \(5 \times 10^{-7}\) \\
Minimum learning rate & \(2 \times 10^{-6}\) \\
Learning rate schedule & cosine decay \\
Warm-up iterations     & \vst{},\vista{} $=$ $7K$, $10K$\\
Total iterations      & \vst{},\vista{} $=$ $70K$, $100K$\\
Batch size            & 1 \\ \bottomrule
\end{tabular}
\caption{\textbf{LoRA and Training Parameters}}
\label{tab:hyperparameters}
\end{table}
